# Supplementary material for: Direct observation of current-induced nonlinear spin torque in Pt-Py bilayers
Source: arXiv:2308.11156 source file (2024-06-17)
Supplement: Supplementary file 1 [file Supplemental_TK24PRB.pdf]

SUPPLEMENTAL MATERIALS

# Direct observation of current-induced nonlinear spin torque in Pt-Py bilayers

Toshiyuki Kodama,[1,*] Nobuaki Kikuchi,[2] Takahiro Chiba,[3]
Satoshi Okamoto,[2,4] Seigo Ohno,[5] and Satoshi Tomita[1,5,†]

[1]Institute for Excellence in Higher Education, Tohoku University, Sendai, 980-8576, Japan
[2]Institute of Multidisciplinary Research for Advanced Materials, Tohoku University, Sendai 980-8577, Japan
[3]Frontier Research Institute for Interdisciplinary Sciences, Tohoku University, Sendai 980-8578, Japan
[4]Center for Science and Innovation in Spintronics, Tohoku University, Sendai 980-8577, Japan
[5]Department of Physics, Graduate School of Science, Tohoku University, Sendai 980-8578, Japan

CONTENTS

**SM1. Effect of substrate on temperature elevation and ST-FMR signal-to-noise ratio**

**SM2. Effect of Pt-Py strip length on the ST-FMR results**

**SM3. Evaluation of Oersted fields generated by the dc current and field-like-torque effective field generated by spin current**

**SM4. Evaluation of electrical current density in Pt layer**

## SM1. Effect of substrate on temperature elevation and ST-FMR signal-to-noise ratio

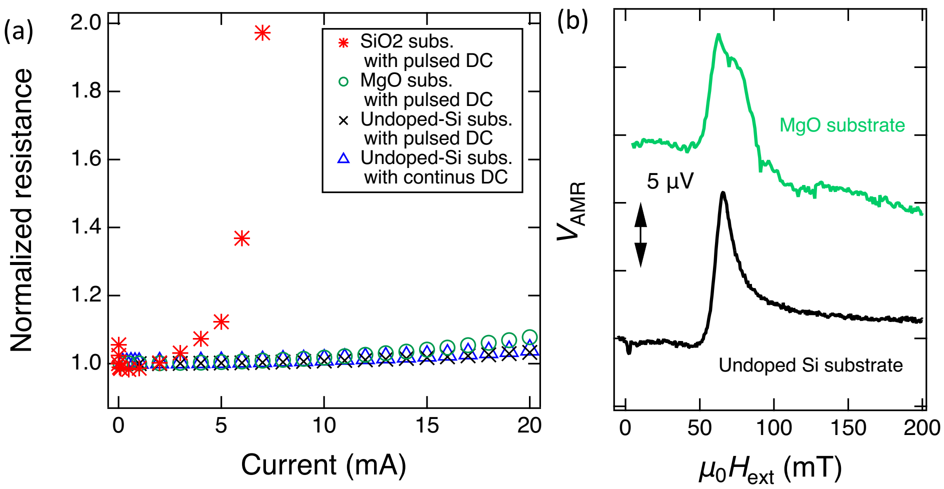


**Fig. S1** (a) Normalized electrical resistance-current curves of specimens on quartz (red asterisks), MgO (green circles), and undoped Si substrates (black crosses). Electrical resistance is normalized by the value at 0.2 mA. The current is chopped at 0.2 ms. A normalized resistance-current curve measured with continuous current is also plotted for the specimen with the undoped Si substrate (blue triangles). (b) ST-FMR signal of the specimens with MgO (green) and undoped Si substrates (black).

Figure S1(a) shows normalized electrical resistance–current curves of Pt-Py bilayer samples with three different substrates: quartz (red asterisks), MgO (green circles), and undoped Si substrate (black crosses). The thermal conductivities of quartz, MgO, and undoped Si are 1.4 W/mK [1], 56 W/mK [2], and 150 W/mK [3], respectively. A chopped dc current at 0.2 ms is used for the measurement. The normalized resistance–current curve of the specimen on the quartz substrate shows a nonlinear increase in resistance, indicating that temperature is elevated significantly in the specimen due to the low thermal conductivity. Contrastingly, the other specimens with MgO and undoped Si substrates highlight a linear increase of resistance, indicating that temperature elevation is small. An additional plot by blue triangles corresponds to a normalized resistance–current curve of the specimen on the undoped Si substrate measured using continuous dc current. The normalized resistance–current curve using continuous current (black crosses) shows a very similar to that using chopped current. Figure S1(b) shows ST-FMR signals probed by $V_{AMR}$ of the specimens with MgO (green) and undoped Si substrate (black). The specimen with the undoped Si substrate demonstrates a high signal-to-noise (S/N) ratio of the $V_{AMR}$ thanks to a better thermal conductivity, while the

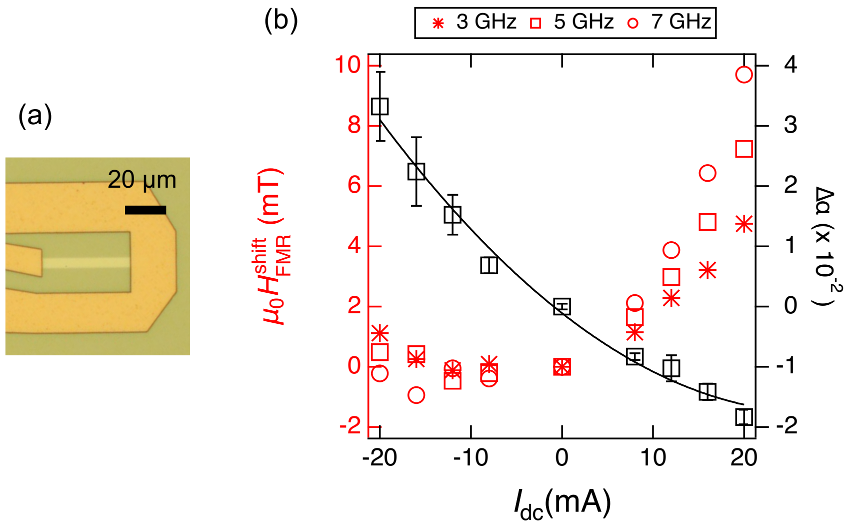


**Fig. S2** (a) Photograph of lithographically-prepared specimen with a longer Pt-Py strip of 45 μm length. (b) Resonance field shift (red asterisks, squares, and circles) and damping parameter variation (black squares) as a function of $I_{dc}$.

specimen on the MgO substrate shows a low S/N ratio.

## SM2. Effect of Pt-Py strip length on the ST-FMR results

ST-FMR measurements are conducted for a specimen with a much longer Py-Pt strip of 45 μm length. Figure S2(a) shows the specimen photograph. The width of the strip is 5  μm. The ST-FMR measurements at various $I_{ac}$ frequency are conducted using $I_{dc}$ between -20 and +20 mA. Figure 2(b) shows the resonance field shift $\mu_0 H_{FMR}^{shift}$ and damping parameter variation $\Delta\alpha$ as a function of $I_{ac}$. Figure S2(b) is very similar to Fig. 2 in the main text. The longer Py-Pt strip reproduces the two striking features discussed in the main text, i.e., i) $\mu_0 H_{FMR}^{shift}$ and $\Delta\alpha$ are dependent nonlinearly on $I_{dc}$, and ii) a higher $f_{ac}$ results in a larger $\mu_0 H_{FMR}^{shift}$ at the same $I_{dc}$,.

## SM3. Evaluation of Oersted fields generated by the dc current and field-like-torque effective field generated by spin current

The strip width of 5 μm is much larger than the Pt thickness $t_{Pt}$ of 5 nm so that the sample can be regarded as an infinitely wide conducting plate. The Oersted field $H_{Oe}$ is calculated using the Ampere's law as $\mu_0 H_{Oe} = J_{Pt} t_{Pt}/2$.

At $I_{dc} = 20$ mA, i.e., $J_{Pt} = 6.5 \times 10^{11}$ A/m$^2$ (See SM4 in the following), $\mu_0 H_{Oe}$ is thus calculated to be $-2.1$ mT. Because Fig.4 in the main text shows $\mu_0 H_{in} = -3.3$ mT at $I_{dc} = 20$ mA, $\mu_0 H_{FLT} + \mu_0 H_{Oe}$ is evaluated to be $-4.6$ mT from $\mu_0 H_{FLT} + \mu_0 H_{Oe} = \mu_0 H_{in} \times \sin^{-1}(\pi/4) = -3.3 \times \sin^{-1}(\pi/4) = -4.6$ mT. Therefore, $\mu_0 H_{FLT} = -4.6 - (-2.1) = -2.5$ mT. This value of $\mu_0 H_{FLT}$ is similar to the transverse effective field of $-1.6$ mT previously reported in Ref. [4].

## SM4. Evaluation of electrical current density in Pt layer

The film thicknesses of Pt, Py and Ta are 5, 2 and 3 nm, respectively. Since the strip width is 5 μm, cross sections of Pt, Py and Ta layers are evaluated to $2.5 \times 10^{-14}$, $1.0 \times 10^{-14}$, and $1.5 \times 10^{-14}$ m$^2$, respectively. Since resistivities of Pt, Py and Ta are respectively $2.0 \times 10^{-7}$, $4.5 \times 10^{-7}$, and $2.1 \times 10^{-6}$ Ωm, the resistance of Pt, Py and Ta layers are $1.9 \times 10^2$, $1.1 \times 10^3$, respectively. If these resistors are connected in parallel, the ratio of current flowing through Pt, Py and Ta layers is evaluated to 1.0 : $1.8 \times 10^{-1}$ : $5.7 \times 10^{-2}$. When dc current of 20 mA is applied, the amount of current flowing in Pt is evaluated to be 16 mA using the ratio of the current flowing in Pt. The 16 mA current in the Pt with cross-section of $2.5 \times 10^{-14}$ m$^2$ yields a current density $6.5 \times 10^{11}$ A/m$^2$. Note that the evaluated current values in the Pt layer are underestimated because the Ta layer is oxidized and becomes an insulator after the deposition on the substrate. The parameters are summarized in the Table S1 below.

TABLE. S1: Evaluated resistance and current ratio in Pt, Py, Ta layers.

| Material | Thickness (m) | Cross section (m$^2$) | Resistivity (Ω m) | Resistance (Ω) | Current ratio |
|---|---|---|---|---|---|
| Pt | $5.0\times 10^{-9}$ | $2.5\times 10^{-14}$ | $2.0\times 10^{-7}$ | $1.9\times 10^{2}$ | 1.0 |
| Py | $2.0\times 10^{-9}$ | $1.0\times 10^{-14}$ | $4.5\times 10^{-7}$ | $1.1\times 10^{3}$ | $1.8\times 10^{-1}$ |
| Ta | $3.0\times 10^{-9}$ | $1.5\times 10^{-14}$ | $2.1\times 10^{-6}$ | $3.4\times 10^{3}$ | $5.7\times 10^{-2}$ |

References

[1] G. A. Slack, Thermal Conductivity of Pure and Impure Silicon, Silicon Carbide, and Diamond, J. Appl. Phys. **35**, 3460 (1964).

[2] W. Zhu, G. Zheng, S. Cao, and H. He, Thermal Conductivity of Amorphous SiO2 Thin Film: A Molecular Dynamics Study, Sci. Rep. **8**, 10537 (2018).

[3] S. Stackhouse, L. Stixrude, and B. B. Karki, Thermal Conductivity of Periclase (MgO) from First Principles, Phys. Rev. Lett. **104**, 208501 (2010).

[4] T. Nan, S. Emori, C. T. Boone, X. Wang, T. M. Oxholm, J. G. Jones, B. M. Howe, G. J. Brown, and N. X. Sun, Comparison of spin-orbit torques and spin pumping526 across NiFe/Pt and NiFe/Cu/Pt interfaces, Phys. Rev. B **91**, 214416 (2015).
